# Supplementary material for: Investigating the parametric dependence of the impact of two-way coupling on inertial particle settling in turbulence
Source: arXiv:2309.07762 source file (2023-09-14)
Supplement: Supplementary file 1 [file A01_timeaverage.tex]

\section{Convergence of time averaged fluid velocity at particle positions}
\label{app_derivation}
